# Supplementary material for: Hydropower optimization: an industrial approach
Source: arXiv:1610.10057 source file (2016-10-31)
Supplement: Supplementary file 1 [file TOOL.tex]

\documentclass{article}
\usepackage{graphicx}
\usepackage{epstopdf}
\usepackage[english]{babel}
\epstopdfsetup{update} % only regenerate pdf files when eps file is newer

\begin{document}
	\includegraphics[scale=0.4]{Real_data} % loads sine-eps-converted-to.pdf
\end{document}
